# Supplementary material for: Loading and relaxation dynamics of a red blood cell
Source: arXiv:2102.08752 ancillary file (2021-05-31)
Supplement: Supplementary file 1 [file esi.pdf]

# Electronic Supplementary Information for: Loading and relaxation dynamics of a red blood cell

**Fabio Guglietta**
Department of Physics & INFN, *University of Rome "Tor Vergata"*[*]
Chair for Computational Analysis of Technical Systems (CATS), *RWTH Aachen University*[†]
Computation-based Science and Technology Research Center, *The Cyprus Institute*[‡]
fabio.guglietta@roma2.infn.it

**Marek Behr**
Chair for Computational Analysis of Technical Systems (CATS), *RWTH Aachen University*[†]

**Giacomo Falcucci**
Department of Enterprise Engineering "Mario Lucertini," *University of Rome "Tor Vergata"*[§]

**Mauro Sbragaglia**
Department of Physics & INFN, *University of Rome "Tor Vergata"*[*]

[*]Via della Ricerca Scientifica 1, 00133, Rome, Italy
[†]52056 Aachen, Germany
[‡]20 Konstantinou Kavafi Str., 2121 Nicosia, Cyprus
[§]Via del Politecnico 1, 00133, Rome, Italy

## 1 Movies

Four movies showing the loading-relaxation simulations for all three kinds of mechanical loads simulated are available. We report here their name and a short description:

- STS: stretching simulation with $F = 50 \times 10^{-12}$ N and $\mu_{\mathrm{m}} = 3.18 \times 10^{-7}$ m Pa s (see Sec. 3.1 in main paper).
- SHS: shear simulation with $\dot{\gamma} = 123$ s$^{-1}$ and $\mu_{\mathrm{m}} = 3.18 \times 10^{-7}$ m Pa s (see Sec. 3.2 in main paper).
- SHS_mum0: shear simulation with $\dot{\gamma} = 123$ s$^{-1}$ and $\mu_{\mathrm{m}} = 0$ m Pa s (see Sec. 3.2 in main paper).
- FRMS: four-roll mill simulation with $\dot{\gamma}_{\mathrm{FRMS}} = 10$ s$^{-1}$ and $\mu_{\mathrm{m}} = 3.18 \times 10^{-7}$ m Pa s (see Sec. 3.3 in main paper).

## 2 Shear simulation (SHS): characteristic time $t_{\mathrm{L}}^{\cos}$

In Fig. 1, values of $t_{\mathrm{L}}^{\cos}$ are reported (see Eq. (13) in main paper) as a function of the shear rate $\dot{\gamma}$ for different values of membrane viscosity $\mu_{\mathrm{m}}$. While $t_{\mathrm{L}}$ measures the time the membrane takes to reach the average deformation $D_{\mathrm{av}}$, the characteristic time $t_{\mathrm{L}}^{\cos}$ measures the period of the oscillations.

## 3 Characteristic times as a function of the average deformation

In Fig. 2 we report the characteristic times $t_{\mathrm{L}}$ and $t_{\mathrm{R}}$ (see Eqs. (12)-(14) in main paper) as well as the ratio $\tilde{t} = t_{\mathrm{L}}/t_{\mathrm{R}}$ as a function of the average deformation $D_{\mathrm{av}}$.

## 4 $\delta$ parameter

In Fig. 3 we report the values of the parameter $\delta_{\mathrm{L}}$ and $\delta_{\mathrm{R}}$ used to interpolate $t_{\mathrm{L}}$ and $t_{\mathrm{R}}$, respectively (see Eqs. (12)-(14) in main paper).

## 5 Multiple time scales

We inspected the presence of multiple loading and relaxation times for all three simulations performed (STS, SHS and FRMS). We consider two values of the membrane viscosity (that is $\mu_{\mathrm{m}} = 0$ m Pa s and $\mu_{\mathrm{m}} = 1.59 \times 10^{-7}$ m Pa s) and for each value of $\mu_{\mathrm{m}}$ we consider two values of the external mechanical load: in particular, for the STS (Fig. 4), we report $F = 5 \times 10^{-12}$ N (panels (a-c)) and $F = 70 \times 10^{-12}$ N (panels (b-d)); for the SHS (Fig. 5), $\dot{\gamma} = 1.23$ s$^{-1}$ (panels (a-c)) and $\dot{\gamma} = 123$ s$^{-1}$ (panels (b-d)); for the FRMS (Fig. 6), $\dot{\gamma}_{\mathrm{FRMS}} = 5$ s$^{-1}$ (panels (a-c)) and $\dot{\gamma}_{\mathrm{FRMS}} = 120$ s$^{-1}$ (panels (b-d)). For all three cases, to better compare the loading and relaxation dynamics, we report $1 - \frac{D(t)}{D_{\mathrm{av}}}$ for the loading (red-shaped points) and $\frac{D(t)}{D_{\mathrm{av}}}$ for the relaxation (blue-shaped points), so that both curves start from 1 and go to 0; moreover, we report the two functions $\exp(-t/t_{\mathrm{L}})^{\delta_{\mathrm{L}}}$ (red line) and $\exp(-t/t_{\mathrm{R}})^{\delta_{\mathrm{R}}}$ (blue line).
In Fig. 7, values of $1 - \frac{D(t)}{D_{\mathrm{av}}}$ (loading) and $\frac{D(t)}{D_{\mathrm{av}}}$ (relaxation) are reported for the FRMS with $\dot{\gamma}_{\mathrm{FRMS}} = 5$ s$^{-1}$; the value of membrane viscosity is $\mu_{\mathrm{m}} = 0.64 \times 10^{-7}$ m Pa s.

## 6 Table of physical and dimensionless parameters

In Tab. 1, we report all parameters used in the simulations in both physical and lattice units.

## 7 Table of fitting coefficients

In Tab. 2, we report the values of the coefficients $a_{\mathrm{L}}$, $a_{\mathrm{R}}$, $b_{\mathrm{L}}$ and $b_{\mathrm{R}}$ used to fit $t_{\mathrm{L}}(\mu_{\mathrm{m}})$ and $t_{\mathrm{R}}(\mu_{\mathrm{m}})$ for the STS, SHS and FRMS at some fixed values of the stress $\sigma$. We use linear fits, $t_{\mathrm{L}}^{\mathrm{FIT}} = a_{\mathrm{L}} + b_{\mathrm{L}}\mu_{\mathrm{m}}$ and $t_{\mathrm{R}}^{\mathrm{FIT}} = a_{\mathrm{R}} + b_{\mathrm{R}}\mu_{\mathrm{m}}$, respectively (see Fig. 5 in main paper). Values of $a$ are expressed in [$10^{-3}$ s], while values of $b$ are expressed in [$10^{4}$ m$^{-1}$ Pa$^{-1}$].

## References


[1] T. Krüger, Computer simulation study of collective phenomena in dense suspensions of red blood cells under shear, Springer Science & Business Media, 2012.

[2] S. Suresh, J. Spatz, J. P. Mills, A. Micoulet, M. Dao, C. Lim, M. Beil and T. Seufferlein, Acta biomaterialia, 2005, **1**, 15–30.

[3] G. Gompper and M. Schick, Soft Matter: Lipid Bilayers and Red Blood Cells, Wiley-VCH, 2008.

# 8 Supplementary figures and tables

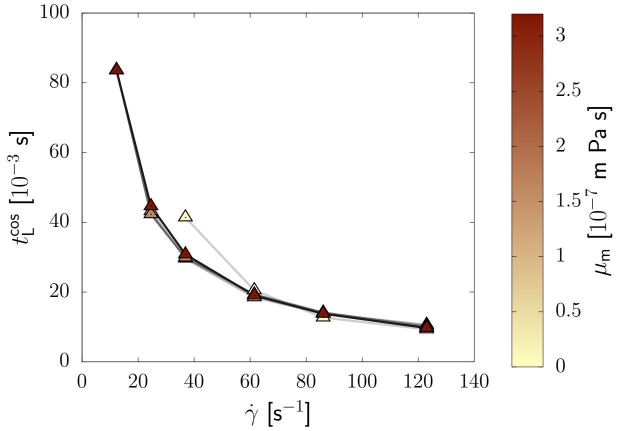


Figure 1: Values of $t_L^{cos}$ as a function of the shear rate $\dot{\gamma}$ (see Eq. (13) in main paper) for different values of membrane viscosity $\mu_m$ (from lightest to darkest color): $\mu_m = 0$ m Pa s (△), $\mu_m = 0.64 \times 10^{-7}$ m Pa s (△), $\mu_m = 1.59 \times 10^{-7}$ m Pa s (▲), $\mu_m = 3.18 \times 10^{-7}$ m Pa s (▲).

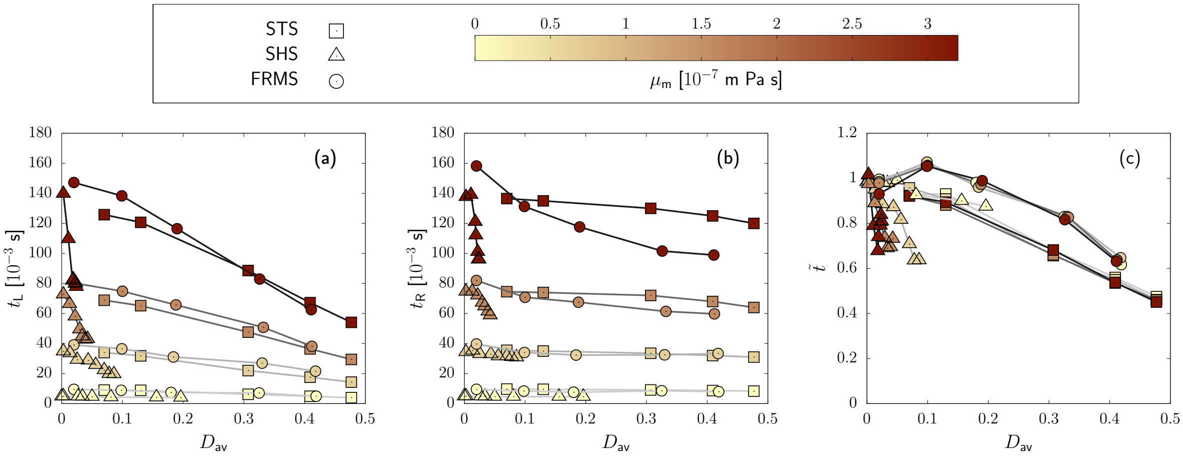


Figure 2: Comparison between the characteristic times $t_L$ (panel (a)), $t_R$ (panel (b)) and the ratio $\tilde{t} = t_L/t_R$ (panel (c)) as a function of the average deformation $D_{av}$ (see Sec. 4 in main paper) for the three simulations performed, i.e., stretching simulation (STS, □), shear simulation (SHS, △), four-roll mill simulation (FRMS, ○), for different values of membrane viscosity $\mu_m$ (from lightest to darkest color): $\mu_m = 0$ m Pa s (□, △, ○), $\mu_m = 0.64 \times 10^{-7}$ m Pa s (□, △, ○), $\mu_m = 1.59 \times 10^{-7}$ m Pa s (■, ▲, ●), $\mu_m = 3.18 \times 10^{-7}$ m Pa s (■, ▲, ●).

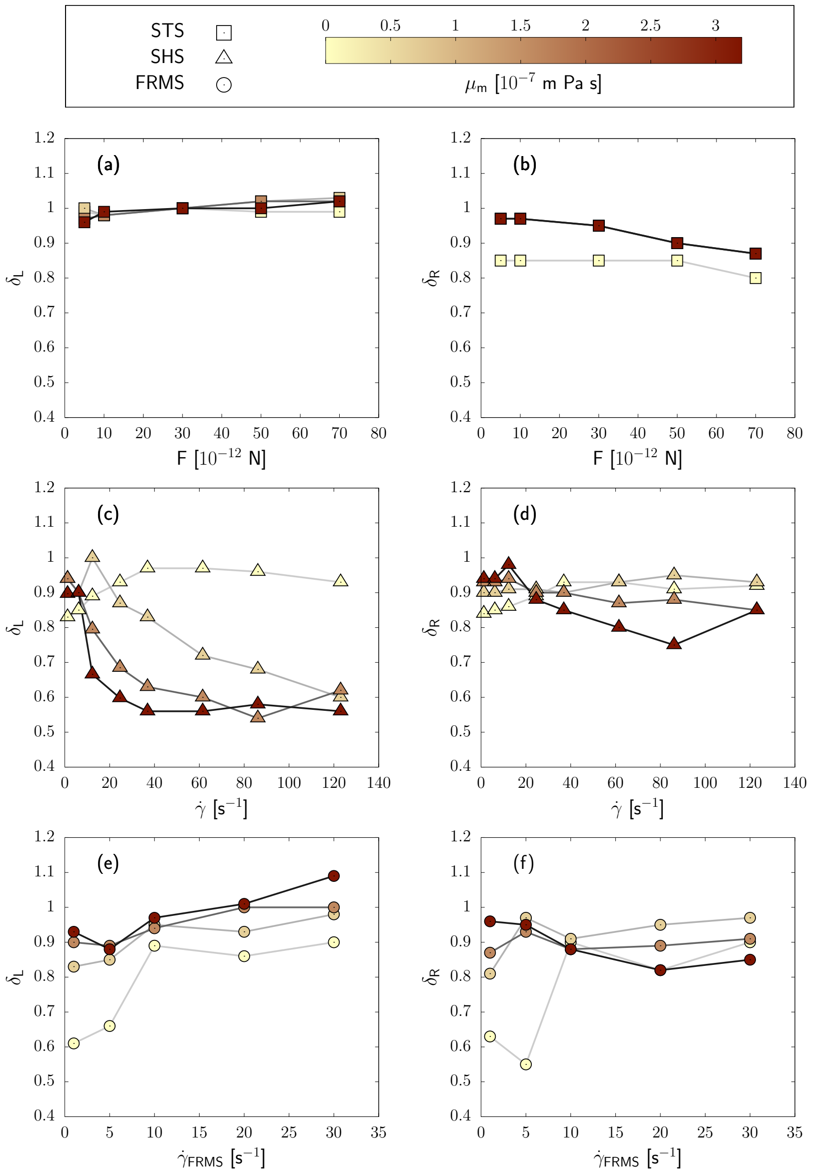


Figure 3: Values of the parameters $\delta_L$ and $\delta_R$ used to interpolate $t_L$, $t_L^{\cos}$ and $t_R$ (see Eqs. (12)-(14) in main paper) are reported for the three simulations performed, i.e., stretching simulation (STS, □, panels (a-b), Sec. 3.1), shear simulation (SHS, △, panels (c-d), Sec. 3.2), four-roll mill simulation (FRMS, ○, panels (e-f), Sec. 3.3), for different values of membrane viscosity $\mu_m$ (from lightest to darkest color): $\mu_m = 0$ m Pa s (□, △, ○), $\mu_m = 0.64 \times 10^{-7}$ m Pa s (□, △, ○), $\mu_m = 1.59 \times 10^{-7}$ m Pa s (■, ▲, ●), $\mu_m = 3.18 \times 10^{-7}$ m Pa s (■, ▲, ●).

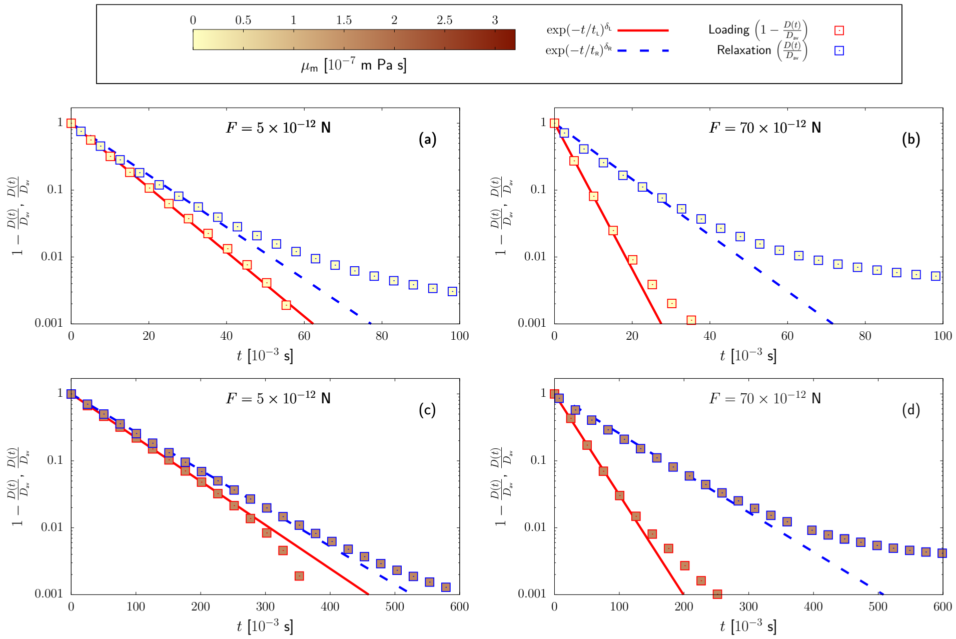


Figure 4: STS: we report the functions $1 - \frac{D(t)}{D_{av}}$ for the loading (□ ■) and $\frac{D(t)}{D_{av}}$ for the relaxation (□ ■). Two values of external force are reported (i.e., $F = 5 \times 10^{-12}$ N (panels (a-c)) and $F = 70 \times 10^{-12}$ N (panels (b-d)); two values of membrane viscosity $\mu_m$ are reported ($\mu_m = 0$ m Pa s (□ □) (panels (a-b)) and $\mu_m = 1.59 \times 10^{-7}$ m Pa s (■ ■) (panels (c-d))). For both loading and relaxation, data are fitted with $\exp(-t/t_L)^{\delta_L}$ (red line) and $\exp(-t/t_R)^{\delta_R}$ (blue line), respectively.

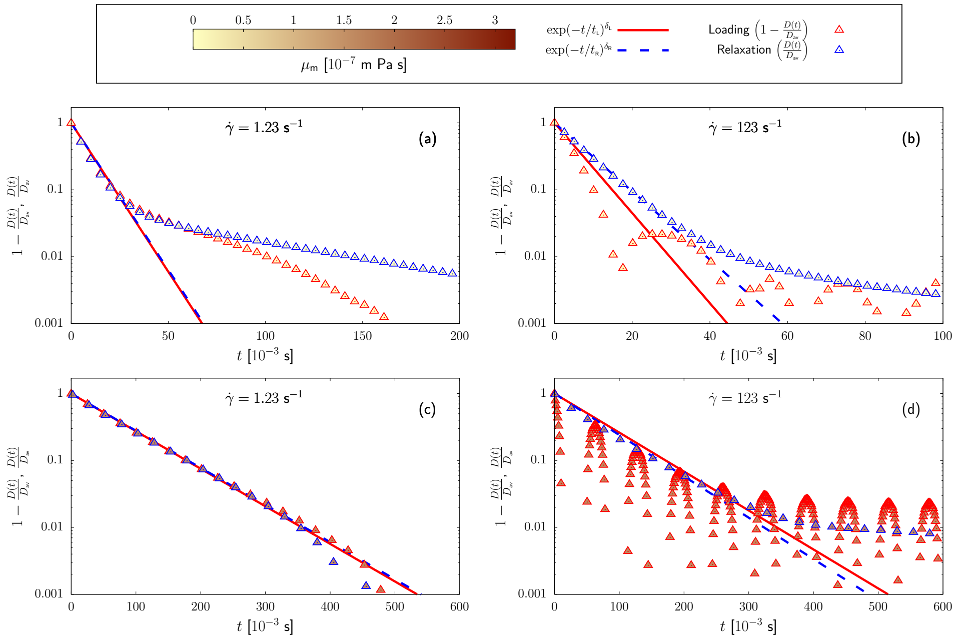


Figure 5: SHS: we report the functions $1 - \frac{D(t)}{D_{av}}$ for the loading (△ ▲) and $\frac{D(t)}{D_{av}}$ for the relaxation (△ ▲. Two values of external force are reported (i.e., $\dot{\gamma} = 1.23$ s$^{-1}$ (panels (a-c)) and $\dot{\gamma} = 123$ s$^{-1}$ (panels (b-d)); two values of membrane viscosity $\mu_m$ are reported ($\mu_m = 0$ m Pa s (△ △) (panels (a-b)) and $\mu_m = 1.59 \times 10^{-7}$ m Pa s (▲ ▲) (panels (c-d))). For both loading and relaxation, data are fitted with $\exp(-t/t_L)^{\delta_L}$ (red line) and $\exp(-t/t_R)^{\delta_R}$ (blue line), respectively.

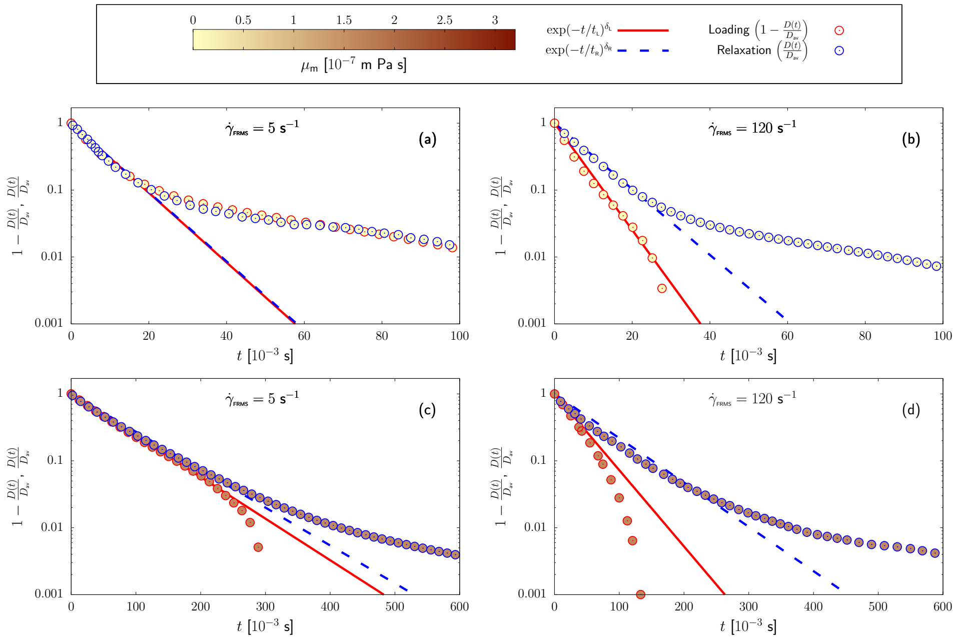

Figure 6: FRMS: we report the functions $1 - \frac{D(t)}{D_{\text{av}}}$ for the loading (○ ●) and $\frac{D(t)}{D_{\text{av}}}$ for the relaxation (○ ●). Two values of external force are reported (i.e., $\dot{\gamma}_{\text{FRMS}} = 5\ \text{s}^{-1}$ (panels (a-c)) and $\dot{\gamma}_{\text{FRMS}} = 120\ \text{s}^{-1}$ (panels (b-d)); two values of membrane viscosity $\mu_{\text{m}}$ are reported ($\mu_{\text{m}} = 0$ m Pa s (○ ○) (panels (a-b)) and $\mu_{\text{m}} = 1.59 \times 10^{-7}$ m Pa s (● ●) (panels (c-d))). For both loading and relaxation, data are fitted with $\exp(-t/t_{\text{L}})^{\delta_{\text{L}}}$ (red line) and $\exp(-t/t_{\text{R}})^{\delta_{\text{R}}}$ (blue line), respectively.

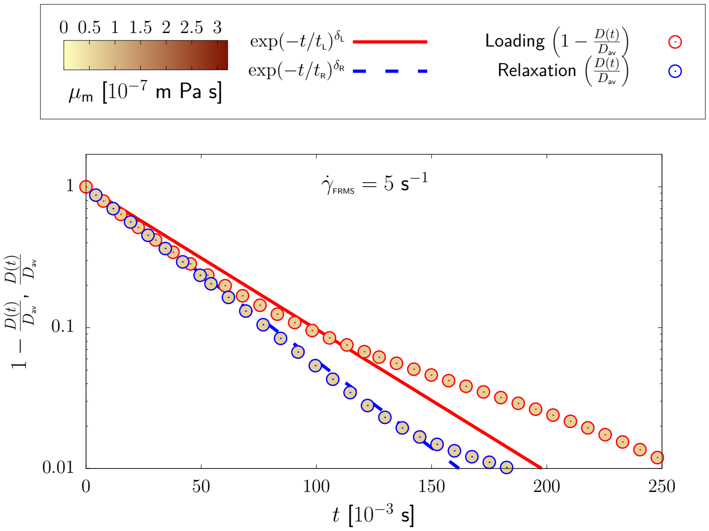

Figure 7: FRMS: we report the functions $1 - \frac{D(t)}{D_{\text{av}}}$ for the loading (●) and $\frac{D(t)}{D_{\text{av}}}$ for the relaxation (●). The value of external force is $\dot{\gamma}_{\text{FRMS}} = 5\ \text{s}^{-1}$; the value of membrane viscosity is $\mu_{\text{m}} = 0.64 \times 10^{-7}$ m Pa s. For both loading and relaxation, data are fitted with $\exp(-t/t_{\text{L}})^{\delta_{\text{L}}}$ (red line) and $\exp(-t/t_{\text{R}})^{\delta_{\text{R}}}$ (blue line), respectively.

| | Physical Units | Lattice Units |
|---|---|---|
| Radius $r$ | $3.91 \times 10^{-6}$ m [1] | $9.78$ |
| Area $A$ | $133 \times 10^{-12}$ m$^2$ | $831$ |
| Volume $V$ | $93 \times 10^{-18}$ m$^3$ | $1453$ |
| Elastic shear modulus $k_{\text{S}}$ (range) | $[5.3, 530] \times 10^{-6}$ Nm$^{-1}$ [2] | $[4.6, 460] \times 10^{-5}$ |
| Elastic dilatational modulus $k_\alpha$ (range) | $[26.5, 2650] \times 10^{-5}$ Nm$^{-1}$ [1] | $[2.30, 230] \times 10^{-3}$ |
| Bending modulus $k_{\text{B}}$ | $2 \times 10^{-19}$ Nm [3] | $1.9 \times 10^{-5}$ |
| Plasma viscosity $\mu_{\text{out}}$ | $1.2 \times 10^{-3}$ Pa s [1] | $0.17$ |
| Cytoplasm viscosity $\mu_{\text{in}}$ | $6 \times 10^{-3}$ Pa s [1] | $0.83$ |
| Membrane viscosity $\mu_{\text{m}}$ (range) | $[0, 3.18] \times 10^{-7}$ m Pa s | $[0, 50]$ |
| Stretching force $F$ used in the STS (range) | $[5, 70] \times 10^{-12}$ N | $[1, 14] \times 10^{-4}$ |
| Shear rate $\dot{\gamma}$ used in the SHS (range) | $[1.23, 123]$ s$^{-1}$ | $[3.09, 309] \times 10^{-8}$ |
| Shear rate $\dot{\gamma}_{\text{FRMS}}$ used in the FRMS (range) | $[1, 30]$ s$^{-1}$ | $[2.52, 75.6] \times 10^{-8}$ |

Table 1: Parameters used in the simulations are reported in both physical and lattice units.

| | | STS | | SHS | | FRMS | |
|---|---|---|---|---|---|---|---|
| | | L | R | L | R | L | R |
| $\sigma = 0.001$ Pa | a | $10.7 \pm 1.3$ | $10.2 \pm 0.4$ | $5.9 \pm 1.1$ | $6.7 \pm 1.5$ | $10.9 \pm 1.1$ | $9.4 \pm 1.1$ |
| | b | $37.5 \pm 0.7$ | $40.0 \pm 0.2$ | $42.4 \pm 0.6$ | $41.6 \pm 0.8$ | $43.4 \pm 0.6$ | $47.9 \pm 0.6$ |
| $\sigma = 0.01$ Pa | a | $9.9 \pm 0.8$ | $10.2 \pm 0.6$ | $9.8 \pm 4.6$ | $6.3 \pm 1.4$ | $10.5 \pm 1.0$ | $9.2 \pm 0.6$ |
| | b | $36.3 \pm 0.4$ | $39.6 \pm 0.3$ | $29.4 \pm 2.5$ | $41.4 \pm 0.7$ | $42.2 \pm 0.5$ | $44.1 \pm 0.3$ |
| $\sigma = 0.025$ Pa | a | $8.8 \pm 0.2$ | $9.9 \pm 0.8$ | $9.4 \pm 4.0$ | $7.3 \pm 2.0$ | $9.8 \pm 0.8$ | $9.0 \pm 0.6$ |
| | b | $33.8 \pm 0.1$ | $39.1 \pm 0.4$ | $23.8 \pm 2.0$ | $34.6 \pm 1.1$ | $40.0 \pm 0.5$ | $38.0 \pm 0.4$ |
| $\sigma = 0.05$ Pa | a | $6.8 \pm 0.2$ | $9.8 \pm 1.0$ | $6.6 \pm 2.2$ | $8.1 \pm 3.0$ | $8.9 \pm 1.7$ | $9.7 \pm 2.2$ |
| | b | $28.1 \pm 0.1$ | $38.1 \pm 0.6$ | $23.6 \pm 1.0$ | $33.3 \pm 1.7$ | $33.4 \pm 0.9$ | $33.9 \pm 1.2$ |
| $\sigma = 0.075$ Pa | a | $5.6 \pm 0.2$ | $9.4 \pm 0.8$ | $5.4 \pm 0.9$ | $9.6 \pm 4.0$ | $9.6 \pm 2.3$ | $10.9 \pm 2.6$ |
| | b | $23.4 \pm 0.1$ | $37.3 \pm 0.5$ | $23.4 \pm 0.5$ | $29.1 \pm 2.0$ | $27.9 \pm 1.2$ | $31.0 \pm 1.5$ |
| $\sigma = 0.1$ Pa | a | $5.0 \pm 0.2$ | $8.9 \pm 0.5$ | $4.4 \pm 0.3$ | $10.0 \pm 5.0$ | $10.0 \pm 2.7$ | $12.0 \pm 3.1$ |
| | b | $19.5 \pm 0.1$ | $36.4 \pm 0.3$ | $23.7 \pm 0.2$ | $28.0 \pm 3.0$ | $22.8 \pm 1.5$ | $28.6 \pm 1.7$ |
| $\sigma = 0.125$ Pa | a | $4.5 \pm 0.2$ | $8.6 \pm 0.2$ | $4.6 \pm 0.7$ | $9.6 \pm 4.5$ | $8.7 \pm 2.6$ | $12.1 \pm 3.4$ |
| | b | $17.0 \pm 0.1$ | $35.4 \pm 0.1$ | $23.2 \pm 0.4$ | $27.9 \pm 2.4$ | $19.7 \pm 1.4$ | $28.1 \pm 1.8$ |

Table 2: Coefficients $a_{\text{L}}$, $a_{\text{R}}$, $b_{\text{L}}$ and $b_{\text{R}}$ used to fit $t_{\text{L}}(\mu_{\text{m}})$ and $t_{\text{R}}(\mu_{\text{m}})$ for the STS, SHS and FRMS at some fixed values of the stress $\sigma$. We use linear fits, $t_{\text{L}}^{\text{FIT}} = a_{\text{L}} + b_{\text{L}}\mu_{\text{m}}$ and $t_{\text{R}}^{\text{FIT}} = a_{\text{R}} + b_{\text{R}}\mu_{\text{m}}$, respectively (see Fig. 5 in main paper). Values of $a$ are expressed in [$10^{-3}$ s], while values of $b$ are expressed in [$10^4$ m$^{-1}$ Pa$^{-1}$].
